# Supplementary material for: MLOD: Awareness of Extrinsic Perturbation in Multi-LiDAR 3D Object Detection for Autonomous Driving
Source: arXiv:2010.11702 source file (2020-09-29)
Supplement: Supplementary file 1 [file appendix.tex]

\textit{\textbf{Problem:}} Given three point clouds ($\mathcal{P}_{1}, \mathcal{P}_2, \mathcal{P}_{3}, \mathbf{p}_n\in\mathbb{R}^{3}$) captured at the same time, output a series of bounding boxes $\mathcal{B}=\big\{\mathbf{b}_{i}\big\}$,
\begin{equation}
	\mathbf{b}_{i} = \big[cls, x, y, z, w, h, l, rz, score\big]
\end{equation}

\textbf{SVM:} 
\begin{equation}
	\begin{split}
		\text{min\ \ } & \frac{1}{2}||\mathbf{w}||^{2} \\
		\text{s.t.\ \ } & y^{(\ell)}(\mathbf{w}^{\top}\mathbf{x}^{(\ell)})+w_{0} \geq 1, \ \ j\forall \ell
	\end{split}
\end{equation}

By introducing slack variables,
\begin{equation}
	\begin{split}
		\text{min\ \ } & \frac{1}{2}||\mathbf{w}||^{2} + C\sum_{i=1}^{N}\xi_{i}\\\	
		\text{s.t.\ \ } &
		y^{(\ell)}(\mathbf{w}^{\top}\mathbf{x}^{(\ell)})+w_{0} \geq 1-\xi_{(\ell)},\ \  \xi_{(\ell)}\geq 0
	\end{split}
\end{equation}

Inference:
\begin{equation}
\mathbf{y}^{*} = \mathbf{w}^{\top}\phi(\mathbf{x},\mathbf{y})
\end{equation}

\textbf{Structured SVM:} allows training of a classifier for general structured output labels.
\begin{equation}
	\begin{split}
		\underset{\mathbf{w}\in\mathbb{R}^{D}}{\text{min}}\ \ &
		\frac{1}{2}||\mathbf{w}||^{2} + \frac{C}{N}\sum_{i=1}^{N}\xi_{i}\\
		\text{s.t.}\ \ &\mathbf{w}^{\top}(\phi(\mathbf{x}^{(\ell)}, \mathbf{y}) - \phi(\mathbf{x}^{(\ell)}, \mathbf{y}^{(\ell)}))
		\geq 
		\Delta(\mathbf{y}^{(\ell)},\mathbf{y})-\xi_{i}, \forall\mathbf{y} \backslash \mathbf{y}^{(\ell)}
	\end{split}
\end{equation}
where $\phi: \mathcal{X}\times\mathcal{Y}\rightarrow \mathbb{R}^{D}$ is a feature function, $\Delta:\mathcal{Y}\times\mathcal{Y}\rightarrow \mathbb{R}_{+}, \Delta(\mathbf{y},\mathbf{z})\geq 0$ measures a distance in label space, the objective function is differentiable.

Than, the best bounding box can be inferred as
\begin{equation}
	\mathbf{y}^{*} = \underset{\mathbf{y}\in\mathcal{Y}}{\text{argmin }}\mathbf{w}^{\top}\phi(\mathbf{x},\mathbf{y})
\end{equation}
