# Supplementary material for: MLOD: Awareness of Extrinsic Perturbation in Multi-LiDAR 3D Object Detection for Autonomous Driving
Source: arXiv:2010.11702 source file (2020-09-29)
Supplement: Supplementary file 2 [file supplementary.tex]

\begin{table}[b]
	\centering
	\caption{Network Details of Stage-One Network}
	\label{tab.network1_details}

	\begin{tabular}{ccccc}
		\hline \toprule[0.03cm]
		Block Name                   & Layer Name            & \begin{tabular}[c]{@{}c@{}}Kernel Size/ \\ Output Unit\end{tabular} & Strides     & Filter \\ \hline \toprule[0.03cm]
		FLN                 & Mean            &N/A                                           & N/A          & N/A   \\ \hline \toprule[0.01cm]
		\multirow{8}{*}{ML} & Subm-Conv3D $\times$2 & {[}3,3,3{]}                                                        & {[}1,1,1{]} & 16     \\
		& Sparse-Conv3D         & {[}3,3,3{]}                                                        & {[}2,2,2{]} & 32     \\
		& Subm-Conv3D $\times$2 & {[}3,3,3{]}                                                        & {[}1,1,1{]} & 32     \\
		& Sparse-Conv3D         & {[}3,3,3{]}                                                        & {[}2,2,2{]} & 64     \\
		& Subm-Conv3D $\times$3 & {[}3,3,3{]}                                                        & {[}1,1,1{]} & 64     \\
		& Sparse-Conv3D         & {[}3,3,3{]}                                                        & {[}2,2,2{]} & 64     \\
		& Subm-Conv3D $\times$3 & {[}3,3,3{]}                                                        & {[}1,1,1{]} & 64     \\
		& Sparse-Conv3D         & {[}3,1,1{]}                                                        & {[}2,1,1{]} & 64     \\ \hline \toprule[0.01cm]
		\multirow{9}{*}{RPN}         & Conv2D                & {[}3,3{]}                                                          & {[}2,2{]}   & 128    \\
		& Conv2D$\times$3       & {[}3,3{]}                                                          & {[}1,1{]}   & 128    \\
		& TransConv2D                & {[}3,3{]}                                                          & {[}1,1{]}   & 256    \\
		& Conv2D                & {[}3,3{]}                                                          & {[}2,2{]}   & 128    \\
		& Conv2D$\times$5       & {[}3,3{]}                                                          & {[}1,1{]}   & 128    \\
		& TransConv2D                & {[}2,2{]}                                                          & {[}2,2{]}   & 256    \\
		& Conv2D                & {[}3,3{]}                                                          & {[}2,2{]}   & 256    \\
		& Conv2D$\times$5       & {[}3,3{]}                                                          & {[}1,1{]}   & 256    \\
		& TransConv2D                & {[}4,4{]}                                                          & {[}4,4{]}   & 256    \\ \hline \toprule[0.01cm]
		Prob-Map                     & Conv2D                & {[}1,1{]}                                                          & {[}1,1{]}   & 2      \\
		Reg-Map                      & Conv2D                & {[}1,1{]}                                                          & {[}1,1{]}   & 16     \\ \hline \toprule[0.03cm]
	\end{tabular}
\end{table}

\begin{table}[b]
	\centering
	\caption{Network Details of Stage-Two Network}
	\label{tab.network2_details}

	\begin{tabular}{cccc}
		\hline \toprule[0.03cm]
		Block Name                & Layer Name & Output Unit  & Filter \\ \hline \toprule[0.03cm]
		\multirow{7}{*}{PointNet} & STN-3      & {[}3,3{]}    & N/A    \\
		& Conv1d     & {[}N,64{]}    & 64     \\
		& STN-64     & {[}64, 64{]} & N/A    \\
		& Conv1d     & {[}N,128{]}   & 128    \\
		& Conv1d     & {[}N,1024{]} & 1024   \\
		& Max-Pool   & {[}1,1024{]} & N/A    \\
		& Concat     & {[}1,1035{]} & N/A    \\ \hline \toprule[0.01cm]
		\multirow{3}{*}{FC-Cls}   & FC-cls1   & {[}1,512{]}  & 512    \\
		& FC-cls2   & {[}1,256{]}  & 256    \\
		& FC-cls3   & {[}1,1{]}    & 1      \\ \hline \toprule[0.01cm]
		\multirow{3}{*}{FC-Reg}   & FC-reg1   & {[}1,512{]}  & 512    \\
		& FC-reg2   & {[}1,256{]}  & 256    \\
		& FC-reg3   & {[}1,8{]}    & 8      \\ \hline \toprule[0.03cm]
	\end{tabular}
\end{table}

\begin{table*}[]
	\centering
	\caption{Mean and Variance of Accuracy ($\text{AP}_{\text{3D}}\ \text{IoU}\geqslant0.7$) under Different Level of Uncertainties (with Fixed Uncertainty Priors)}

	\begin{tabular}{@{}ccccccccccccc@{}}
		\toprule[0.03cm]
		\multirow{2}{*}{Cases} & \multicolumn{3}{c}{$\alpha = 0$}              & \multicolumn{3}{c}{$\alpha = 0.02$}                                & \multicolumn{3}{c}{$\alpha = 0.04$}                                & \multicolumn{3}{c}{$\alpha = 0.1$}                                 \\
		& \textit{easy}          & \textit{mod.}          & \textit{hard}          & \textit{easy}                 & \textit{mod.}                 & \textit{hard}                 & \textit{easy}                 & \textit{mod.}                 & \textit{hard}                 & \textit{easy}                 & \textit{mod.}                 & \textit{hard}                 \\ \toprule[0.03cm]
		\textit{Top LiDAR}           & 63.3          & 53.8          & 38.2          & 63.3                 & 53.8                 & 38.2                 & 63.3                 & 53.8                 & 38.2                 & 63.3                 & 53.8                 & 38.2                 \\ \toprule[0.03cm]
		\textit{Input Fusion}        & 71.2          & \textbf{62.3} & \textbf{45.4} & 64.7 $\pm$ 2.5          & 60.8 $\pm$ 0.4          & 44.4 $\pm$ 0.2          & \textbf{63.0} $\pm$ 0.5 & 53.9 $\pm$ 2.1          & \textbf{38.0} $\pm$ 0.2 & 60.9 $\pm$ 1.0          & \textbf{51.0} $\pm$ 0.6 & \textbf{36.1} $\pm$ 0.4   \\
		\textit{MLOD-I}              & \textbf{71.6} & 61.9          & \textbf{45.4} & \textbf{64.8} $\pm$ 2.4 & \textbf{61.2} $\pm$ 0.4 & \textbf{44.6} $\pm$ 0.3 & 62.9 $\pm$ 0.5          & \textbf{57.0} $\pm$ 3.3 & 37.7 $\pm$ 0.3          & \textbf{61.2} $\pm$ 0.8 & 50.9 $\pm$ 0.5          & 35.8 $\pm$ 0.4          \\ \toprule[0.01cm]
		\textit{Input Fusion (OC)}   & -			 & -             & -             & 66.8 $\pm$ 4.0          & 61.2 $\pm$ 0.5          & 44.5 $\pm$ 0.2          & 63.4 $\pm$ 0.4          & 60.0 $\pm$ 0.5          & 42.8 $\pm$ 2.2          & 62.4 $\pm$ 0.6          & 52.3 $\pm$ 0.4          & \textbf{37.2} $\pm$ 0.2 \\ 
		
		\textit{MLOD-I (OC)}         & -			 & -             & -             & \textbf{67.7} $\pm$ 3.9 & \textbf{61.4} $\pm$ 0.4 & \textbf{44.8} $\pm$ 0.2 & \textbf{64.2} $\pm$ 2.5 & \textbf{60.4} $\pm$ 0.6 & \textbf{43.0} $\pm$ 2.5 & \textbf{62.5} $\pm$ 0.5 & \textbf{52.3} $\pm$ 0.3 & 36.9 $\pm$ 0.3          \\ \toprule[0.03cm]
		
		\textit{Feature Fusion}      & 71.2          & 59.2          & 42.9          & 63.9 $\pm$ 2.5          & 59.2 $\pm$ 0.9          & 42.9 $\pm$ 0.9          & 62.9 $\pm$ 0.4          & 58.6 $\pm$ 2.5          & \textbf{41.1} $\pm$ 3.3 & 61.9 $\pm$ 0.6          & 51.1 $\pm$ 1.0          & 35.7 $\pm$ 0.7          \\ 
		\textit{MLOD-F}              & \textbf{71.8} & \textbf{60.9} & \textbf{44.5} & \textbf{65.4} $\pm$ 3.3 & \textbf{60.7} $\pm$ 0.4 & \textbf{44.3} $\pm$ 0.3 & \textbf{63.7} $\pm$ 0.5 & \textbf{59.7} $\pm$ 2.1 & 40.5 $\pm$ 2.8          & \textbf{63.2} $\pm$ 0.5 & \textbf{53.1} $\pm$ 0.6 & \textbf{37.7} $\pm$ 0.3 \\ \toprule[0.01cm]
		
		\textit{Feature Fusion (OC)} & -			 & -             & -             & 66.2 $\pm$ 3.7          & 59.5 $\pm$ 0.8          & 43.5 $\pm$ 0.9          & 63.8 $\pm$ 2.2          & 59.6 $\pm$ 0.7          & 43.6 $\pm$ 0.7          & 63.3 $\pm$ 2.4          & 54.3 $\pm$ 3.0          & 37.9 $\pm$ 2.0          \\
		\textit{MLOD-F (OC)}         & -			 & -             & -             & \textbf{67.1} $\pm$ 3.7 & \textbf{60.9} $\pm$ 0.3 & \textbf{44.4} $\pm$ 0.2 & \textbf{65.3} $\pm$ 3.1 & \textbf{60.6} $\pm$ 0.4 & \textbf{44.1} $\pm$ 0.2 & \textbf{64.4} $\pm$ 2.2 & \textbf{57.6} $\pm$ 3.2 & \textbf{39.2} $\pm$ 2.3 \\ \toprule[0.03cm]
		
		\textit{Result Fusion}       & 70.4          & \textbf{62.1} & 44.0          & 64.5 $\pm$ 2.3          & 60.1 $\pm$ 0.4          & 43.4 $\pm$ 0.2          & 63.0 $\pm$ 0.5          & 55.5 $\pm$ 2.9          & 38.1 $\pm$ 0.2          & 61.1 $\pm$ 1.0          & 51.5 $\pm$ 0.5          & 36.8 $\pm$ 0.3          \\
		\textit{MLOD-R}              & \textbf{71.3} & 61.4          & \textbf{44.4} & \textbf{66.9} $\pm$ 3.7 & \textbf{60.6} $\pm$ 0.4 & \textbf{44.0} $\pm$ 0.3 & \textbf{63.1} $\pm$ 0.4 & \textbf{59.2} $\pm$ 0.4 & \textbf{38.9} $\pm$ 2.2 & \textbf{62.2} $\pm$ 0.8 & \textbf{52.2} $\pm$ 0.4 & \textbf{37.1} $\pm$ 0.2 \\ \toprule[0.01cm]
		
		\textit{Result Fusion (OC)}  & -			 & -             & -             & 66.5 $\pm$ 3.7          & 60.4 $\pm$ 0.6          & 43.5 $\pm$ 0.2          & 64.0 $\pm$ 2.2          & 59.3 $\pm$ 0.4          & 42.0 $\pm$ 1.9          & 62.5 $\pm$ 0.6          & 52.5 $\pm$ 0.4          & 37.5 $\pm$ 0.2          \\
		\textit{MLOD-R (OC)}         & -			 & -             & -             & \textbf{66.8} $\pm$ 3.7 & \textbf{60.9} $\pm$ 0.4 & \textbf{44.1} $\pm$ 0.2 & \textbf{64.3} $\pm$ 2.5 & \textbf{59.9} $\pm$ 0.6 & \textbf{43.0} $\pm$ 1.7 & \textbf{63.0} $\pm$ 0.5 & \textbf{52.8} $\pm$ 0.4 & \textbf{37.4} $\pm$ 0.2 \\ \toprule[0.03cm]
	\end{tabular}
	\label{tab.robust_test_fixed_prior}
\end{table*}

\section{Supplementary Materials}
\subsection{Sensitivity Analyze of Extrinsic Uncertainty}

The stage-2 input of \textit{MLOD} consists of the uncertainty, which is propagated through \eqref{equ.uncertainty_of_each_point} 
with an extrinsic perturbation prior $\bm{\Theta}$ and the scaling parameter $\alpha$.
The scale of $\alpha$ can be given by manual or estimated via online system identification.
In this section, we study the sensitivity of \textit{MLOD} to the precision of $\alpha$.
In order to do so, we conduct another robustness evaluation, which is similar to Section \ref{sec:experiment_ruc}.
Instead of testing with the ground-truth $\alpha$, we only use the fixed $\alpha=0.06$ as the stage-2 input.
The results are shown in Tab. \ref{tab.robust_test_fixed_prior}.
The same conclusion hold for the cases with a fixed uncertainty prior to their ground-truth counterparts.
By comparing with Tab. \ref{tab.robust_test},
the cases with a fixed uncertainty prior perform comparable accuracies as their ground-truth counterparts.
In other words, it shows that the proposed \textit{MLOD} is able to handle the inaccurate $\alpha$ situation.

\subsubsection{Stage One}
The network details of stage one are shown in Tab. \ref{tab.network1_details}.
Each Subm-Conv3D / Sparse-Conv3D block in the Middle Layers (ML) includes a 3D sub-manifold convolution layer/ 3D Sparse convolution layer, a batch normalization layer and a ReLU layer sequentially.
The Conv2D / TransConv2D block in the region proposal network (RPN) consists of a 2D convolution layer / 2D transpose convolution layer, a ReLU layer and a batch normalization layer.
The model of the Probability Map and Regression Map is an individual 2D convolution layer.

We voxelize the point clouds with a resolution $[0.05, 0.05, 0.14]m$ in the range $[-35.2, -40, -5.7]m$ to $[35.2, 40, 2]m$.
The anchors are set as $[1.8, 4.5, 1.6]m$ in terms of the average size of car samples in the training set.
Two anchors with $[0, 90]^{\circ}$ are set at each position.
In the training stage, we use batch size as $3$ for all stage one and the single-LiDAR cases.
The learning rate is initialized as $2.25\times 10^{-3}$ and applied the warm-up methods in the whole $50$ epochs.

\subsubsection{Stage Two}
The details of the proposed stage-2 network are shown in Tab. \ref{tab.network2_details}.
The STN-3 and STN-64 represent the STN Network used in \cite{qi2017pointnet}.
We encode the sore of each proposal into a One-hot vector.
It combines with the parameter of each proposal to form the extra feature, as described in Section \ref{sec:methodology}.
Each Conv1d in the PointNet consists of a 1D convolution layer, a batch normalization layer and a ReLU layer
Except for the last layer, FC-cls and FC-reg layers consist of a fully connected layer, a batch normalization layer, and a ReLU layer.

In the training stage, we use batch size at $128$.
The learning rate is initialized as $2.25\times 10^{-3}$ and applied warm-up methods in the whole 50 epochs.

\subsection{More details about Network and Training}
Here we report the training details of car class since it has the majority of samples  in the LYFT multi-LiDAR dataset,
and the proposed method could be extended to other categories (like pedestrian and cyclist)
easily with little modifications of hyperparameters.

\subsection{Qualitative Results}
Here we demonstrate more qualitative results for visualization in Fig \ref{fig.qual_vis_all}.
It is noted that we sample the extrinsic perturbation for all the cases at the 3-sigma position according to $\bm{\Theta}$ for comparison.
It demonstrates that \textit{MLOD} trusts more on certain points and 
refines the proposals according to the propagated uncertainties.

\begin{figure*}[]
	\centering
	\includegraphics[width=0.85\textwidth]{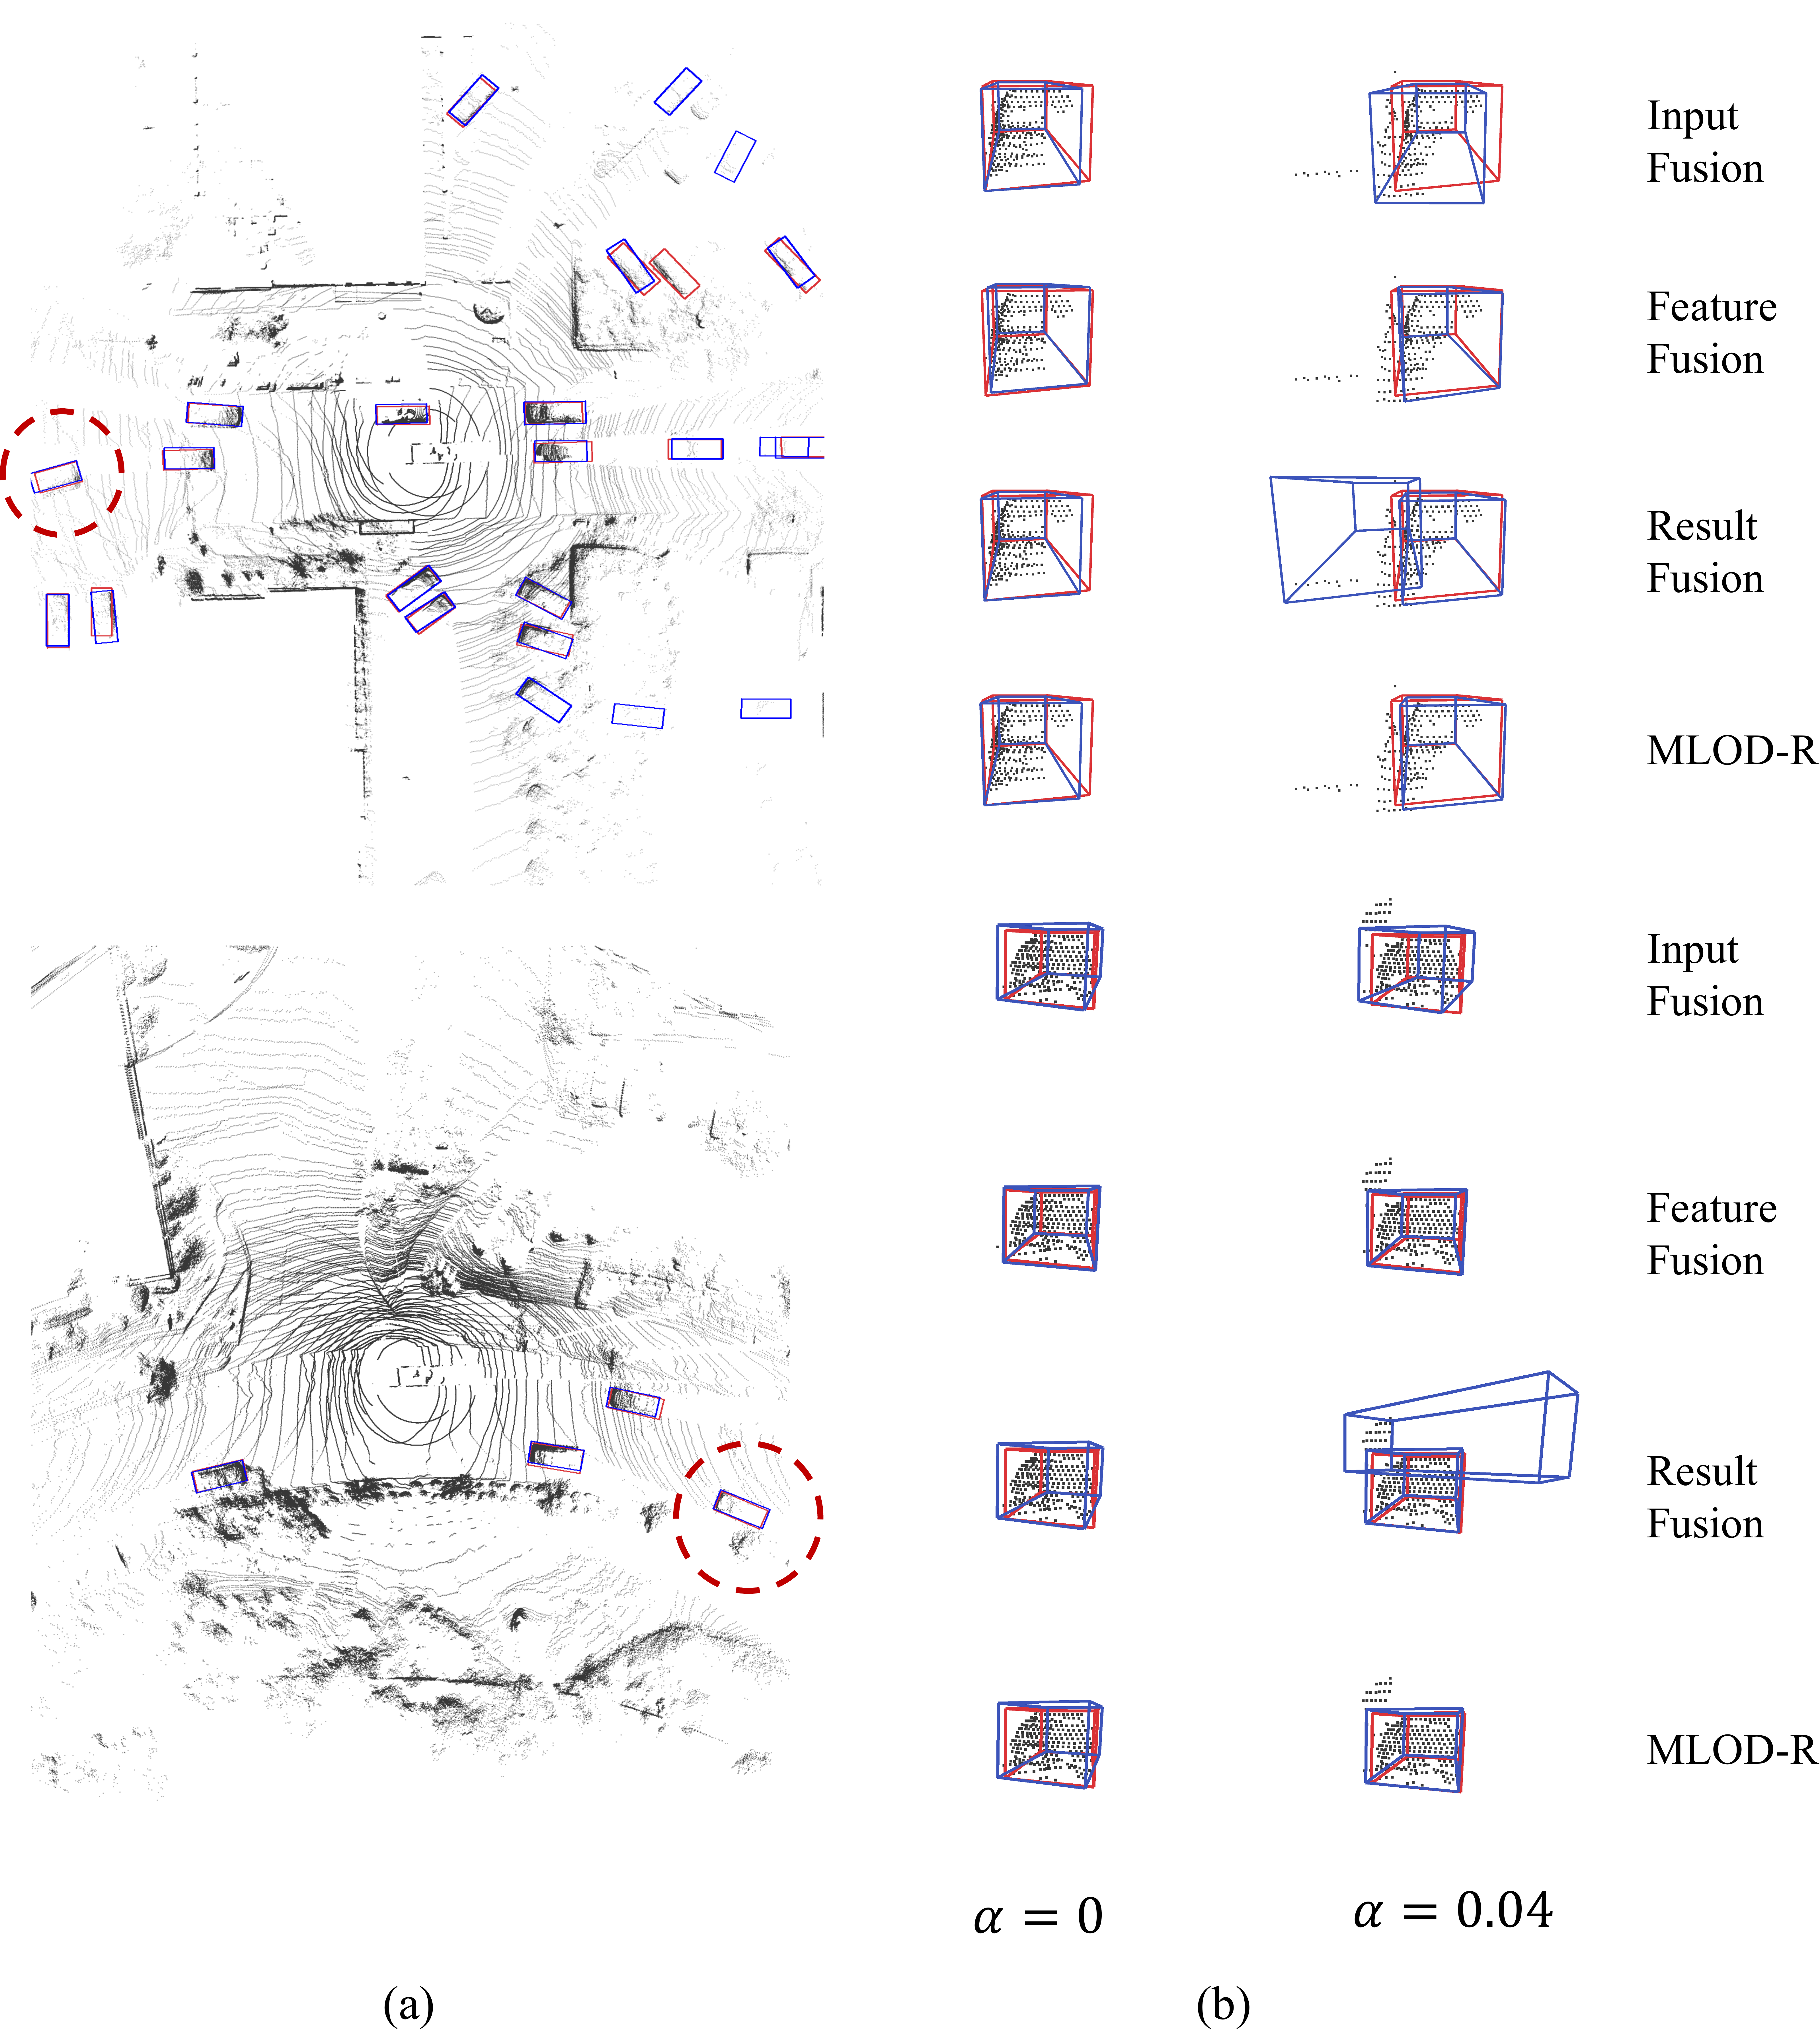}
	\caption{Visualization of the fusion schemes results
    (For comparison, here we sample the extrinsic perturbation for all the ($\alpha=0.04$) cases at the $\sigma$ position according to $\bm{\Theta}$.
    (a) Bird's-eye view of \textit{MLOD}'s detection results when $\alpha=0.04$.
    The extrinsic perturbation is observed from where the red arrows indicate.
    (b) A close-up view of results estimated by different fusion schemes within the red circle. Left to right: $\alpha=0$, $\alpha=0.04$.
    \textit{Input Fusion}, \textit{Feature Fusion} and \textit{Result Fusion} suffer from false positives or inaccurate boxes caused by extrinsic perturbation and inaccurate box location.
    Compared with its counterpart (\textit{Result Fusion}), \textit{MLOD-R} eliminates the false positives and refines the 3D boxes.
	}
	\label{fig.qual_vis_all}
\end{figure*}
