# Supplementary material for: MLOD: Awareness of Extrinsic Perturbation in Multi-LiDAR 3D Object Detection for Autonomous Driving
Source: arXiv:2010.11702 source file (2020-09-29)
Supplement: Supplementary file 3 [file supplementary_material.tex]

\section{Supplementary Material}

\subsection{Dataset Details}
We provide the detailed parameters of CARLA for data collection in Tab. \ref{tab.carla_setup}. The whole dataset cover four episodes with different starting points. In each episode, $2000$ frames are collected, and we remove the start frames, so $7944$ frames in total are used for training and evaluation. 

\begin{figure*}
	\centering
	\includegraphics[width=0.66\textwidth]{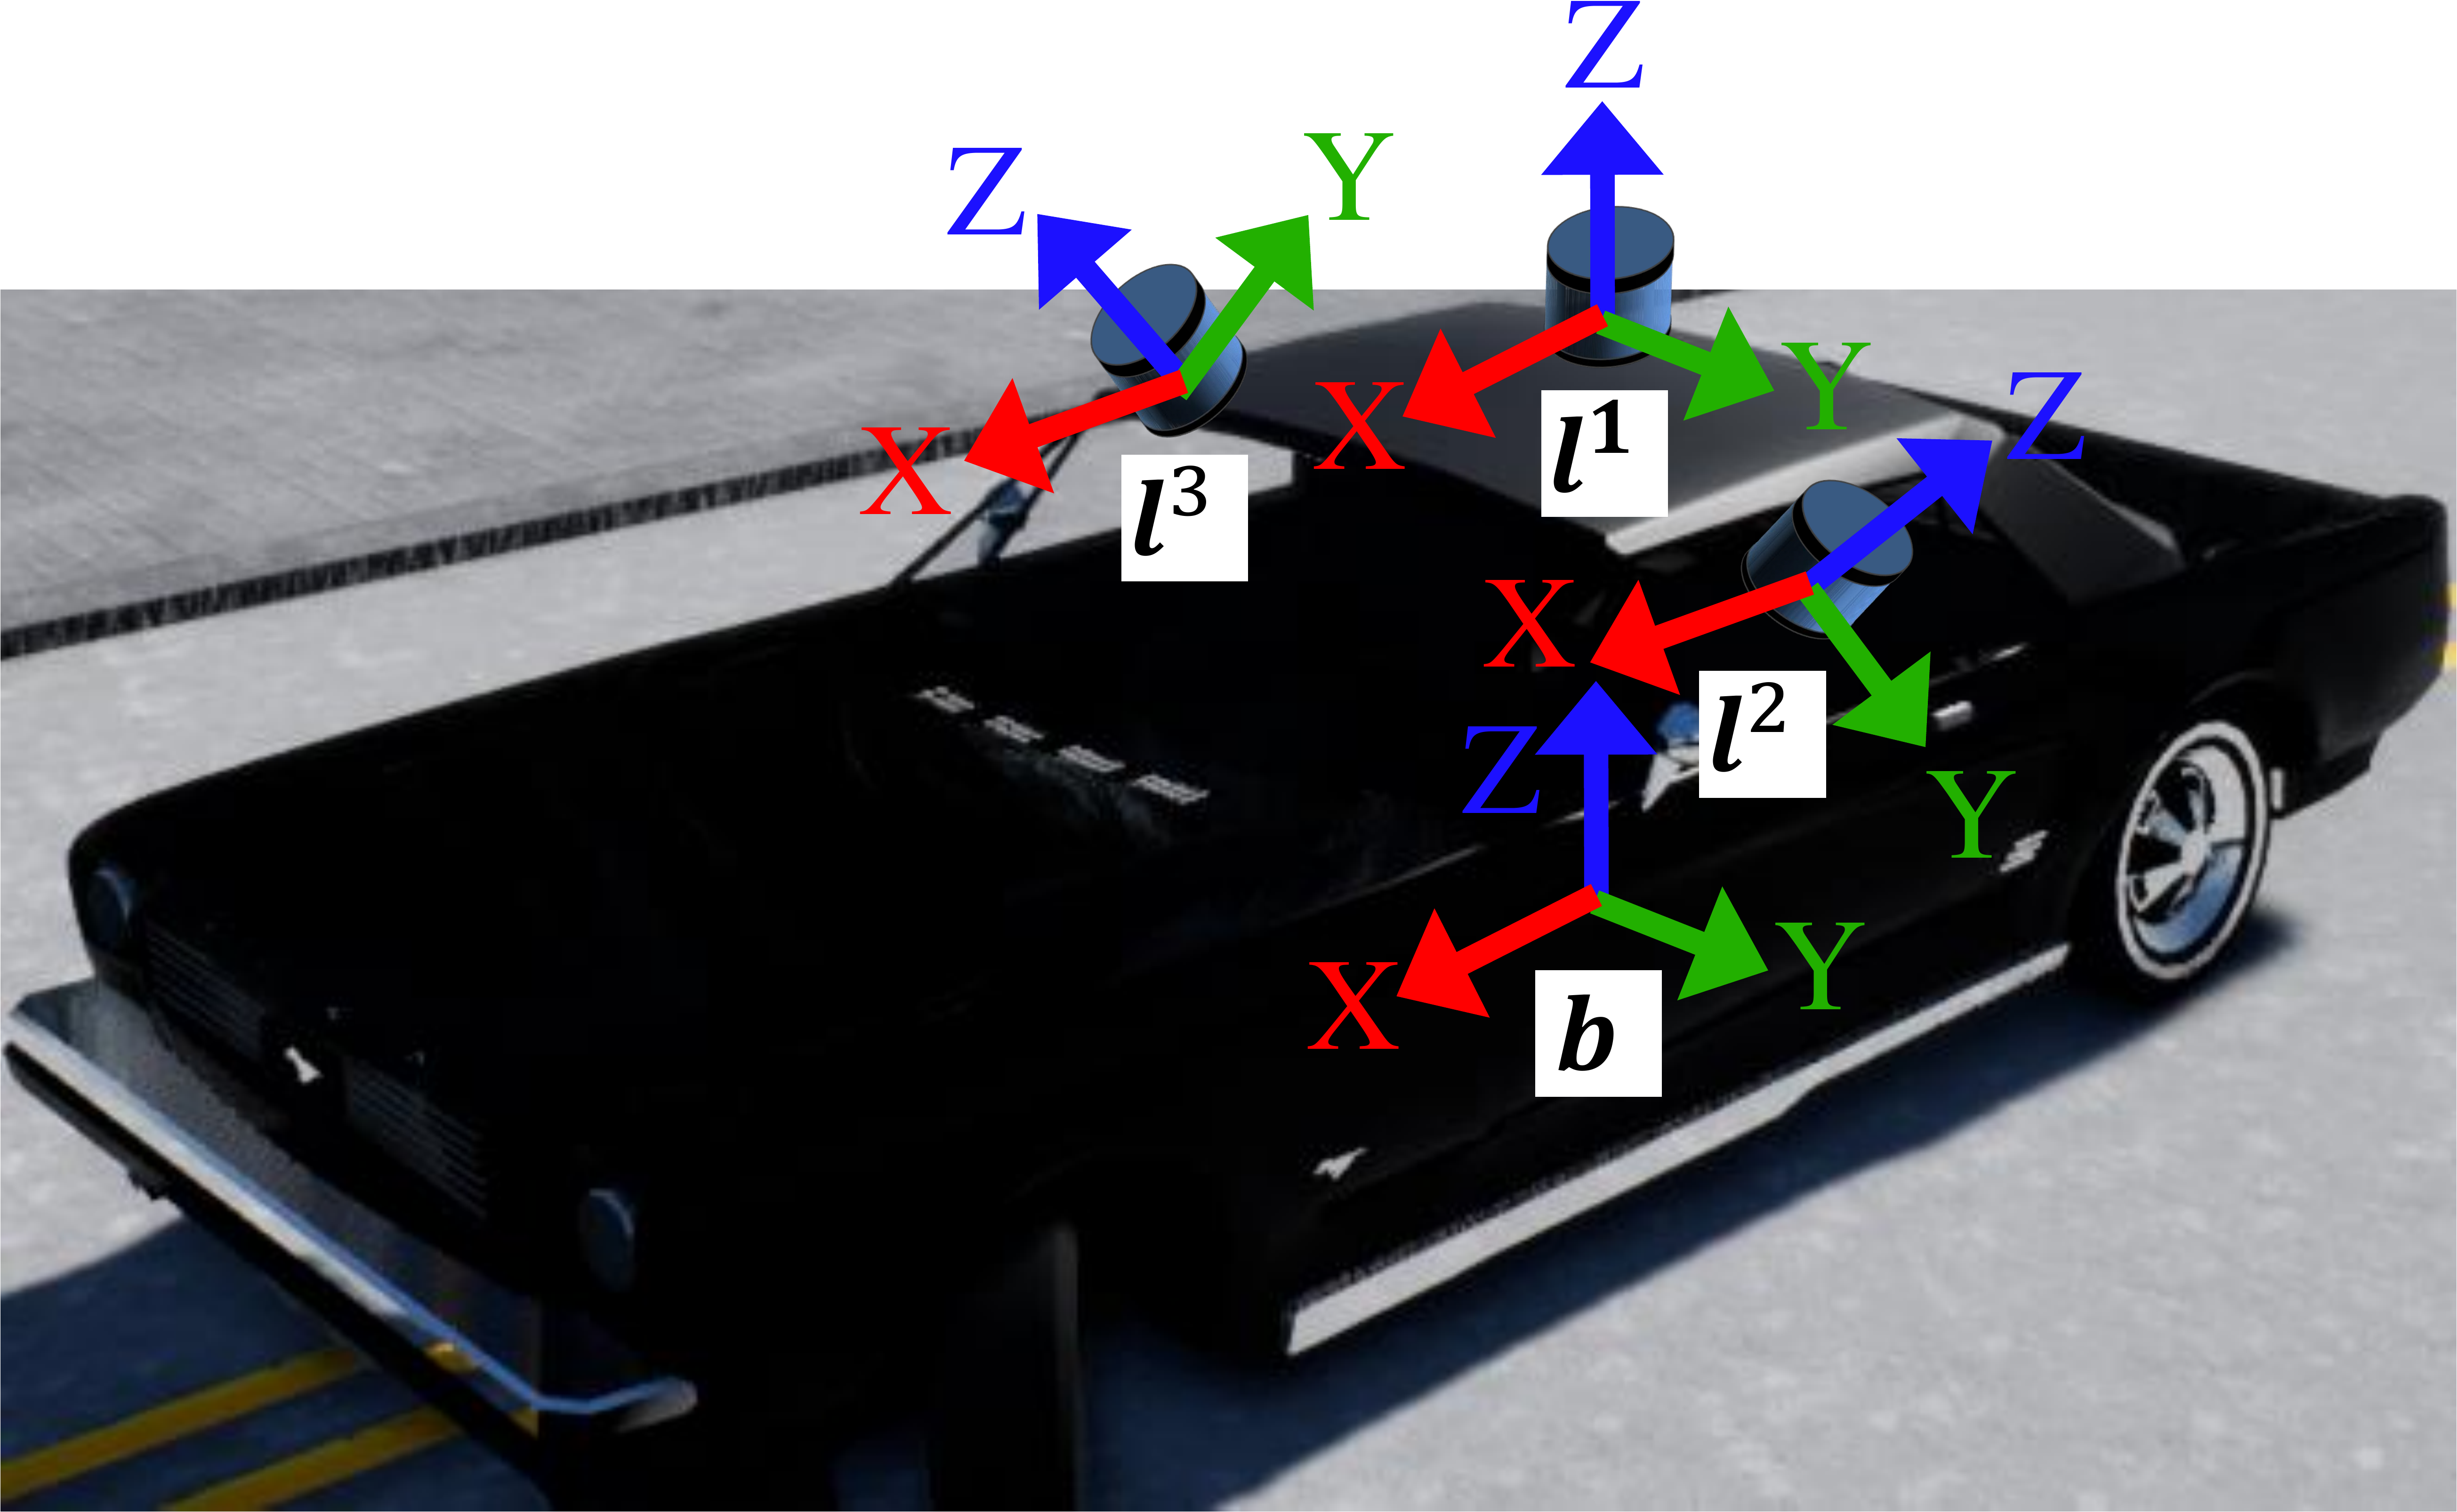}
	\caption{The multi-LiDAR setup on the vehicle in CARLA.}  
	\label{fig.carla_car}    
\end{figure*}  

\begin{table*}[tph]
	\centering  	
	\begin{tabular}{ccccc}
		\hline
		\toprule[0.03cm] 
		Episode & Total Frame & $N_{\text{vehicle}}$ & $N_{\text{pedestrain}}$ 
		&\begin{tabular}[c]{@{}c@{}}LiDAR property\\ (range[m], points/s, hz, vertical FOV)\end{tabular}
		\\ \hline \toprule[0.03cm]
		4       & 7944            & 90               & 60                  & $100,\ 250000,\ 10,\ +2 \text{ to } 24.8^{\circ}$ \\ 
		\hline
		\toprule[0.03cm] 
	\end{tabular}
	\caption{The CARLA setup.}	
	\label{tab.carla_setup}       
\end{table*}

We follow \cite{rs_p3} to design the multi-LiDAR setup, which consists of three 64-beam LiDARs mounted on a vehicle. As presented in Fig. \ref{fig.carla_car}, all LiDARs are mounted on the top, and both $l^{2}$ and $l^{3}$ have $30$-degree rotational offsets on the $x\textendash$ axis compared to $l^{1}$. 
Here we use $b\ominus l^{i}$ to represent the configuration from $b$ to $l^{i}$. The extrinsic parameters of different frames are shown in Tab. \ref{tab.real_sensor_setup}.
\begin{table}[tph]
	\centering

	\begin{tabular}{ccccccc}
		\hline
		\toprule[0.03cm] 
		{\multirow{2}{*}{Conf.}} & \multicolumn{3}{c}{Rotation {[}degree{]}}                                               & \multicolumn{3}{c}{Translation {[}m{]}}    \\ \cline{2-7} 
		{}                       & x                         & y                         & z                          & x                          & y                         & z                          \\ \hline \toprule[0.03cm]
		$b\ominus l^{1}$  & 0 & 0 & 0 & 0 & 0 & 2.4 \\ 
		$b\ominus l^{2}$  & -30 & 0 & 0 & 0 & 0.8 & 2.2 \\ 
		$b\ominus l^{3}$  & 30 & 0 & 0 &0 & -0.8 & 2.2  \\                 
		\hline
		\toprule[0.03cm] 
	\end{tabular}    
	\label{tab.real_sensor_setup}   
	\caption{The extrinsic parameters of the multi-LiDAR system.}  	  
\end{table}

\newpage
\subsection{Network Details}
The network details for 3D object detection are shown in Tab. \ref{tab.network_details}. The feature learning network (FLN) consists of a fully connected layer, a batch normalization layer and a ReLU layer sequentially.
Each Subm-Conv3D / Sparse-Conv3D block in the Middle Layers (ML) includes a 3D sub-manifold convolution layer/ 3D Sparse convolution layer, a batch normalization layer and a ReLU layer sequentially. 
The Conv2D block in the region proposal network (RPN) consists of a 2D convolution layer, a ReLU layer and a batch normalization layer.
The model of the Probability Map and Regression Map is an individual 2D convolution layer. We adopt the original parameterization method and residual vector for regression from \cite{zhou2018voxelnet}. 
\begin{table}[tph]
	\begin{center}

		\begin{tabular}{ccccc}
			\hline \toprule[0.03cm] 
			Block Name                   & Layer Name            & \begin{tabular}[c]{@{}c@{}}Kernel Size/ \\ Output Unit\end{tabular} & Strides     & Filter \\ \hline \toprule[0.03cm]
			\multirow{3}{*}{FLN}  & VFE                   & 32                                                                 & N/A         & N/A    \\
			& VFE                   & 128                                                                & N/A         & N/A    \\
			& FCN                    & 128                                                                & N/A         & N/A    \\ \hline \toprule[0.01cm]
			\multirow{8}{*}{ML} & Subm-Conv3D $\times$2 & {[}3,3,3{]}                                                        & {[}1,1,1{]} & 16     \\
			& Sparse-Conv3D         & {[}3,3,3{]}                                                        & {[}2,2,2{]} & 32     \\
			& Subm-Conv3D $\times$2 & {[}3,3,3{]}                                                        & {[}1,1,1{]} & 32     \\
			& Sparse-Conv3D         & {[}3,3,3{]}                                                        & {[}2,2,2{]} & 64     \\
			& Subm-Conv3D $\times$3 & {[}3,3,3{]}                                                        & {[}1,1,1{]} & 64     \\
			& Sparse-Conv3D         & {[}3,3,3{]}                                                        & {[}2,2,2{]} & 64     \\
			& Subm-Conv3D $\times$3 & {[}3,3,3{]}                                                        & {[}1,1,1{]} & 64     \\
			& Sparse-Conv3D         & {[}3,1,1{]}                                                        & {[}2,1,1{]} & 64     \\ \hline \toprule[0.01cm] 
			\multirow{9}{*}{RPN}         & Conv2D                & {[}3,3{]}                                                          & {[}2,2{]}   & 128    \\
			& Conv2D$\times$3       & {[}3,3{]}                                                          & {[}1,1{]}   & 128    \\
			& DeConv                & {[}3,3{]}                                                          & {[}1,1{]}   & 256    \\
			& Conv2D                & {[}3,3{]}                                                          & {[}2,2{]}   & 128    \\
			& Conv2D$\times$5       & {[}3,3{]}                                                          & {[}1,1{]}   & 128    \\
			& DeConv                & {[}2,2{]}                                                          & {[}2,2{]}   & 256    \\
			& Conv2D                & {[}3,3{]}                                                          & {[}2,2{]}   & 256    \\
			& Conv2D$\times$5       & {[}3,3{]}                                                          & {[}1,1{]}   & 256    \\
			& DeConv                & {[}4,4{]}                                                          & {[}4,4{]}   & 256    \\ \hline \toprule[0.01cm]
			Prob-Map                     & Conv2D                & {[}1,1{]}                                                          & {[}1,1{]}   & 2      \\
			Reg-Map                      & Conv2D                & {[}1,1{]}                                                          & {[}1,1{]}   & 16     \\ \hline \toprule[0.03cm]
		\end{tabular}
	\end{center}
	\label{tab.network_details}
	\caption{Our Implementation Details.}	
\end{table}

\subsection{Qualitative Results}
We also show more qualitatively results from the baseline and three fusion approaches on the validation set of CARLA object detection in Fig. \ref{fig.qualitative_result_supply}.

\begin{figure*}
	\centering
	\includegraphics[width=1\textwidth]{figure/experiment/result_whole-crop.pdf}
	\caption{Another example detection results of MLOD with all fusion schemes on CARLA validation set. From left to right, top to bottom indicates the detection on: $l^{1}$, $l^{2}$, $l^{3}$, input fusion, feature fusion, and result fusion. The detection is in yellow color, while the ground-truth is in purple color. }  
	\label{fig.qualitative_result_supply}  
\end{figure*}
